# Supplementary material for: AURORA:Automated Training Framework of Universal Process Reward Models via Ensemble Prompting and Reverse Verification
Source: arXiv:2502.11520 source file (2025-02-17)
Supplement: Supplementary file 1 [file gene_prompt.tex]

\tcbuselibrary{breakable}

\begin{tcolorbox}[title=default system prompt, label={fig:generate_prompt_default}, breakable]

\textbf{[System]:}\\

\end{tcolorbox}
\begin{tcolorbox}[title=qwq system prompt, label={fig:generate_prompt_qwq}, breakable]

\textbf{[System]:}\\

\end{tcolorbox}
\begin{tcolorbox}[title=inf-o1 $\pi_0$ system prompt, label={fig:generate_prompt_infpi0}, breakable]

\textbf{[System]:}\\

\end{tcolorbox}
